# Supplementary material for: Explaining in Style: Training a GAN to explain a classifier in StyleSpace
Source: arXiv:2104.13369 source file (2021-09-01)
Supplement: Supplementary file 1 [file appendix.tex]

\appendix
\onecolumn

\section{Datasets and classifiers}
\label{appendix:datasets}

For this study we used classifiers on diverse domains, to demonstrate the generality of our method. The list of all datasets is summarized at Table \ref{tab:domains}, and in this section we'll give more details on how they were used. 

\begin{itemize}
    \item{AFHQ \cite{choi2020stargan}}. For Cats / Dogs We trained a binary classifier on the collection of cats and dog faces from AFHQ. For wild cats, we used manual labeling on the subset of images from the "wild" category of AFHQ which contained one of the wild cats - Tiger, Lion, Cheetah, Leopard and Jaguar, and trained a 5-way classifier to predict these labels.
    \item{FFHQ \cite{karras2019style}}. Since FFHQ has no labels, we trained a classifier on the similar CelebA-HQ dataset on the {\it Young} or {\it Male} attributes, and used this classifier for producing labels on FFHQ. 
    \item{Plant-Village \cite{hughes2015open}}. We trained a binary classifier on Healthy vs. Sick leaves, by combining all the labels which contain "healthy" to a single class, and all the other labels to the "sick" class.
    \item{Retinal Fundus \cite{krause2018grader}}. For this dataset, we used the internal grading of DME as described in \cite{krause2018grader}.
    \item{CUB-2011 \cite{wah2011caltech}}. We trained a classifier predicting all 200 classes in the dataset. To 
\end{itemize}

All of the classifiers we trained used the MobileNet architecture, with input size of 512x512 for the Retinal Fundus domains and 256x256 for the rest of the domains.
